# Supplementary material for: Towards Practical Few-Shot Query Sets: Transductive Minimum Description Length Inference
Source: arXiv:2210.14545 source file (2022-10-26)
Supplement: Supplementary file 1 [file appendix.tex]

\appendix
